# Supplementary material for: Triplet-blockaded Josephson supercurrent in double quantum dots
Source: arXiv:2008.04375 ancillary file (2021-01-04)
Supplement: Supplementary file 1 [file supplement.pdf]

# Supplementary Information

# Triplet-blockaded Josephson supercurrent in double quantum dots

Daniël Bouman,[1] Ruben J. J. van Gulik,[1] Gorm Steffensen,[2] Dávid Pataki,[3] Péter Boross,[4] Peter Krogstrup,[2] Jesper Nygård,[2] Jens Paaske,[2] András Pályi,[3] and Attila Geresdi[1,5,*]

[1]*QuTech and Kavli Institute of Nanoscience, Delft University of Technology, NL-2600 GA Delft, The Netherlands*

[2]*Center for Quantum Devices, Niels Bohr Institute, University of Copenhagen, DK-2100 Copenhagen, Denmark*

[3]*Department of Theoretical Physics and MTA-BME Exotic Quantum Phases Research Group, Budapest University of Technology and Economics, H-1111 Budapest, Hungary*

[4]*Institute for Solid State Physics and Optics, Wigner Research Centre for Physics, P.O. Box 49, H-1525 Budapest, Hungary*

[5]*Quantum Device Physics Laboratory, Department of Microtechnology and Nanoscience, Chalmers University of Technology, SE-41296 Gothenburg, Sweden*

## CONTENTS

Device fabrication 3

Estimating electrostatic parameters 3

Switching current measurements 5

Magnetic field dependence of the supercurrent in the even and odd charge sectors 6

Error analysis of the current-phase relationship 7

Supercurrent modeling 8
- Zero-bandwidth approximation 9
- Perturbative expansion of $I_C$ with BCS leads 9

Sign of the critical current to leading order in dot-lead couplings 11
- Sign of all contributions to critical current 13
- Discussion of spin-orbit coupling 16

Simple arguments for triplet blockade 18

Supplementary references 20

* Corresponding author. E-mail address: geresdi@chalmers.se

## DEVICE FABRICATION

The device is fabricated on a commercial undoped Si wafer with a 285 nm thermally grown $SiO_x$ layer with conventional electron beam lithography methods. First, the nanowire is deterministically deposited using a micro manipulator between identification markers [1]. Next, the junctions are defined by etching the aluminum shell for 55 s in a photo developer containing 2% TMAH at room temperature. The wire contacts and the SQUID loop are created by Ar plasma milling and in-situ sputtering of NbTiN.

A 10 nm thick global $AlO_x$ gate dielectric is deposited through a low-temperature thermal atomic layer deposition process. Wrap-around gates with a thickness of approximately 50 nm are deposited in a high-vacuum electron-beam evaporation chamber under three different angles, 60°, 0° and −60° with respect to the normal to ensure conformal coverage. Finally, the $AlO_x$ layer is removed at the wirebond terminals using the same wet etching solution as used for the aluminum shell.

## ESTIMATING ELECTROSTATIC PARAMETERS

We start the characterization in the normal state by quenching superconductivity in the nanowire with a perpendicular magnetic field $B_\perp = 0.5\,\mathrm{T}$ (Fig. S1a). The SQUID reference junction is pinched off and by measuring the conductance at a voltage bias close to zero, we obtain the charge stability diagram of the DQD. The scan is taken around the same gate values as the data in the main text. We estimate the inter-dot lever arms from the slopes of the charge boundaries, shown as white solid lines in Fig. S1a.

Next, we find the lever arm $\alpha_{\mathrm{LL}}$ by comparing the measured height of the Coulomb diamond in Fig. S1b with the width in $V_{\mathrm{L}}$. Combined with inter-dot lever arms, this gives us enough information to estimate the charging energies and relevant capacitances using Eqs. S1 .

$$U_{\mathrm{L}} = \frac{e^2}{C_{\mathrm{L}}}\left(\frac{1}{1-\frac{C_{\mathrm{C}}^2}{C_{\mathrm{L}}C_{\mathrm{R}}}}\right), U_{\mathrm{R}} = \frac{e^2}{C_{\mathrm{R}}}\left(\frac{1}{1-\frac{C_{\mathrm{C}}^2}{C_{\mathrm{L}}C_{\mathrm{R}}}}\right), U_{\mathrm{C}} = \frac{e^2}{C_{\mathrm{C}}}\left(\frac{1}{\frac{C_{\mathrm{L}}C_{\mathrm{R}}}{C_{\mathrm{C}}^2}-1}\right), \tag{S1}$$

where $C_{\mathrm{C}}$ is the inter-dot capacitance and $C_{\mathrm{L(R)}} = C_{\mathrm{BL(BR)}} + C_{V_{\mathrm{L}}(V_{\mathrm{R}})} + C_{\mathrm{C}}$, with $C_{\mathrm{BL(BR)}}$ the capacitance between a dot and the nearest lead and $C_{V_{\mathrm{L}}(V_{\mathrm{R}})}$ the capacitance between a dot and the nearest gate [2]. A complete list of extracted parameters is shown in Table S1. Due

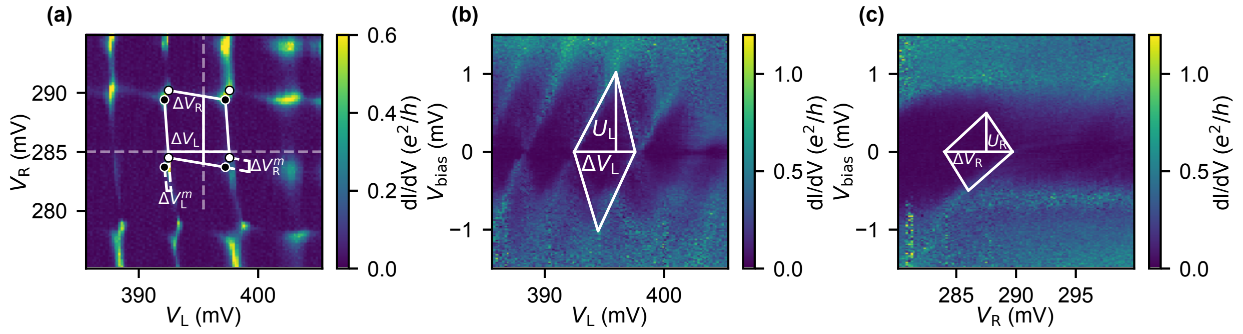


FIG. S1. Normal-state characterization of the DQD. (a) Charge stability diagram taken at $B_\perp = 0.5\,\mathrm{T}$. The ranges of the Coulomb diamond scans in the other subfigures are marked by the dashed lines. (b) Coulomb diamond scan of quantum dot 1 with voltage bias $V_{\mathrm{bias}}$. We extract $\alpha_{\mathrm{LL}} = 0.2, U_{\mathrm{L}} = 1.03\,\mathrm{meV}$. (c) Coulomb diamond scan of quantum dot 2. We verify $U_{\mathrm{R}} = 504\,\mathrm{\mu eV}$.

to the poor visibility of the Coulomb diamond scan of dot 2, we extract $\alpha_{\mathrm{RR}}$ from the other parameters and verify the resulting $U_{\mathrm{R}}$ in Fig. S1c.

TABLE S1. Electrostatic parameters of the DQD device.

| Quantity | Normal state | Superconducting state |
|---|---|---|
| $U_{\mathrm{L}}$ | $1030\,\mathrm{\mu eV}$ | $597\,\mathrm{\mu eV}$ |
| $U_{\mathrm{R}}$ | $504\,\mathrm{\mu eV}$ | $466\,\mathrm{\mu eV}$ |
| $U_{\mathrm{C}}$ | $71\,\mathrm{\mu eV}$ | $42\,\mathrm{\mu eV}$ |
| $\alpha_{\mathrm{LL}}$ | 0.2 | 0.2 |
| $\alpha_{\mathrm{LR}}$ | 0.012 | 0.011 |
| $\alpha_{\mathrm{RL}}$ | 0.014 | 0.013 |
| $\alpha_{\mathrm{RR}}$ | 0.088 | 0.0124 |
| $C_{\mathrm{C}}$ | 0.022 fF | 0.024 fF |
| $C_{\mathrm{L(R)}}$ | 0.157 fF (0.321 fF) | 0.270 fF (0.346 fF) |
| $C_{V_{\mathrm{L}}(V_{\mathrm{R}})}$ | 0.031 fF (0.028 fF) | 0.047 fF (0.039 fF) |
| $C_{\mathrm{BL(BR)}}$ | 0.104 fF (0.271 fF) | 0.199 fF (0.283 fF) |

Due to the non-zero g-factor of the InAs nanowire, the extracted charging energies in the normal state at $B_\perp = 0.5\,\mathrm{T}$ are not the same as in the superconducting state at $B_\perp \approx 0$. Therefore, we extract a separate set of parameters from the superconducting data and

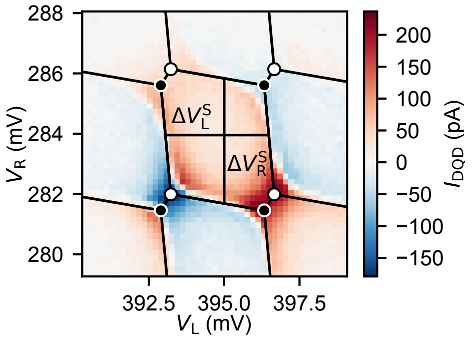


FIG. S2. Superconducting-state characterization. (a) Supercurrent charge stability diagram. The estimated charge-sector boundaries are shown as black solid lines.

only use $\alpha_{\mathrm{LL}} = 0.2$ from the normal state data, while determining all other parameters independently.

The charge state boundaries are identified where $I_{\mathrm{DQD}}$ crosses zero. We overlay the estimated charge boundaries without considering avoided crossings due to the coupling between the quantum dots. We use $\alpha_{\mathrm{LL}} = 0.2$ from the normal-state data and adjust the other parameters such that they agree with the supercurrent stability diagram (Fig. 2). We use these values for the numerical zero-bandwidth calculations shown in the main text. Tab. S1 lists all the electrostatic parameters extracted in the superconducting regime in the rightmost column.

## SWITCHING CURRENT MEASUREMENTS

Due to the stochastic nature of the switching current, we take approximately 20 measurements with a rate of 20 Hz to get a reliable value for a single data point. We use a current bias $I_{\mathrm{bias}}$ with a sawtooth waveform and record $I_{\mathrm{bias}}$ at the point where the voltage $V$ measured over the junction jumps from zero to a finite value. Fig. S3 shows the typical voltage and current waveforms. The blue line is the $I_{\mathrm{bias}}$ signal and the orange line depicts $V$. The red horizontal dashed line indicates the voltage threshold $V_{\mathrm{thres}}$, at which point $I_{\mathrm{bias}}$ is recorded as $I_{\mathrm{SW}}$. Note that the data plotted in this figure was taken on a different device and is used here for the purpose of illustrating the data acquisition method.

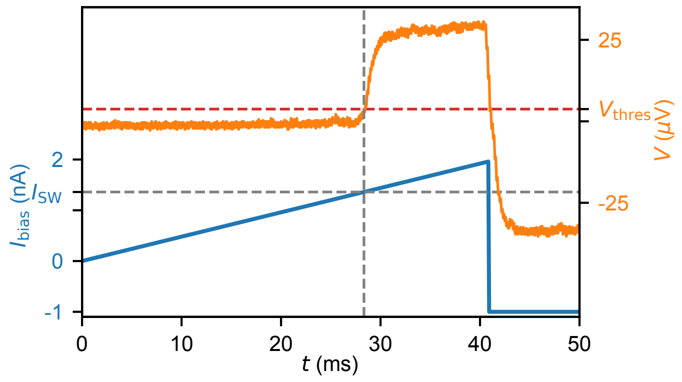


FIG. S3. Switching current measurement protocol to obtain $I_{SW}$. When the measured voltage (orange line) reaches $V_{thres}$ (red horizontal dashed line), the current bias (blue line) is recorded as $I_{SW}$.

## MAGNETIC FIELD DEPENDENCE OF THE SUPERCURRENT IN THE EVEN AND ODD CHARGE SECTORS

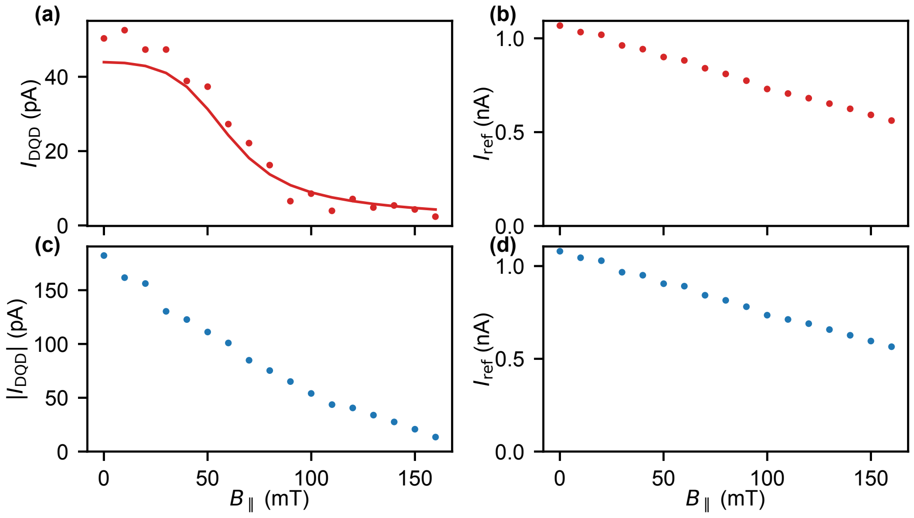


FIG. S4. Extracted switching currents of the DQD and the reference arm as a function of the magnetic field. (a,b) Switching current amplitudes when the DQD is in the even sector. The solid line in subfigure (a) is the same theory fit as in the main text. (c,d) Switching current amplitudes when the DQD is in the odd sector. Panels (a) and (c) display the switching current of the double quantum dot, whereas panels (b) and (d) show the evolution of the reference arm switching current.

The supercurrent through the DQD Josephson junction experiences a global decrease

in amplitude with increasing external magnetic field (see Fig. 3a in the main text). This behavior is qualitatively different from the spin-blockaded supercurrent only seen in the even charge sector. In Fig. S4, we compare the switching current amplitude of both the DQD junction and the reference arm in the even (Fig. S4a,b) and in the odd (Fig. S4c,d) sector. In both cases, the supercurrent through the reference arm $I_{\mathrm{ref}}$ exhibits a gradual decrease as a function of magnetic field. The magnitude of the supercurrent through the DQD $|I_{\mathrm{DQD}}|$ shows similar behavior only in the odd sector (Fig. S4c), while the supercurrent in the even sector decreases strongly around $B_{\|} = 80\,\mathrm{mT}$, clearly distinguishing this behavior from the other cases.

## ERROR ANALYSIS OF THE CURRENT-PHASE RELATIONSHIP

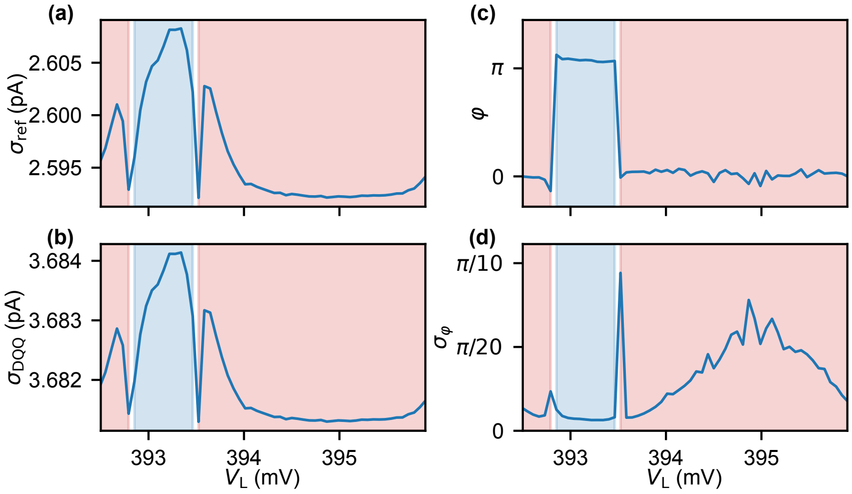


FIG. S5. Supercurrent fit parameter errors. (a) The standard deviation of the reference arm switching current $I_{\mathrm{ref}}$ and (b) that of the DQD junction $I_{\mathrm{DQD}}$. Note that the typical expectation values of these parameters are typically one to two orders of magnitude larger, see the data in the main text. (c) The extracted phase $\varphi$ of the DQD junction and (d) the corresponding standard deviation. The 0 and $\pi$ regions are indicated by a red and blue background, respectively.

## SUPERCURRENT MODELING

In this section, we present the two approaches used to model the critical current $I_\mathrm{C}$, namely a zero-bandwidth (ZBW) approximation and a leading order perturbation theory in dot-lead tunneling amplitude (same approach as in supplement of Ref. [3]). At sufficiently weak coupling and at zero temperature, these two approaches yield a very similar $I_\mathrm{C}$.

We describe the full S-DQD-S system using a serially coupled two-orbital Anderson model with superconducting (BCS) leads:

$$H = H_0 + H_\mathrm{d} + H_\mathrm{SO} + H_\mathrm{BCS} + H_\mathrm{T} \tag{S2}$$

$$H_0 = \sum_{\sigma,i=\mathrm{L,R}} (\epsilon_i + \sigma g_i B) n_{i\sigma} + \sum_{i=\mathrm{L,R}} U_i n_{i\uparrow} n_{i\downarrow} + U_\mathrm{C}(n_{\mathrm{L}\uparrow} + n_{\mathrm{L}\downarrow})(n_{\mathrm{R}\uparrow} + n_{\mathrm{R}\downarrow}) \tag{S3}$$

$$H_\mathrm{d} = t_0 \sum_\sigma (d^\dagger_{\mathrm{L}\sigma} d_{\mathrm{R}\sigma} + d^\dagger_{\mathrm{R}\sigma} d_{\mathrm{L}\sigma}) \tag{S4}$$

$$H_\mathrm{SO} = \sum_{j=x,y,z} \sum_{\sigma,\sigma'} \left( i t_j \tau^j_{\sigma\sigma'} d^\dagger_{\mathrm{L}\sigma} d_{\mathrm{R}\sigma'} - i t_j \tau^j_{\sigma\sigma'} d^\dagger_{\mathrm{R}\sigma} d_{\mathrm{L}\sigma'} \right) \tag{S5}$$

$$H_\mathrm{BCS} = \sum_{k,\sigma,i=\mathrm{L,R}} \xi_i c^\dagger_{ik\sigma} c_{ik\sigma} + \sum_{k,i=\mathrm{L,R}} \left( \Delta_i c^\dagger_{ik\uparrow} c^\dagger_{i-k\downarrow} + \Delta^*_i c_{i-k\downarrow} c_{ik\uparrow} \right) \tag{S6}$$

$$H_\mathrm{T} = \sum_{k,\sigma,i=\mathrm{L,R}} t_i \left( c^\dagger_{ik\sigma} d_{i\sigma} + d^\dagger_{i\sigma} c_{ik\sigma} \right) \tag{S7}$$

Here, $n_{i\sigma}$ denotes the electron occupation operator for dot $i = \mathrm{L,R}$ with spin $\sigma =\uparrow,\downarrow$. $t_x$, $t_y$ and $t_z$ are interdot spin-orbit tunneling amplitudes, and $\tau^j$ is the vector of Pauli matrices [4]. Through the lever arms, the gating will affect $\epsilon_i$ and thereby control the ground state. For this setup, all phases on tunnel couplings $t_0$, $t_\mathrm{L}$ and $t_\mathrm{R}$ can be gauged onto the superconducting order parameter $\Delta_\mathrm{L} = \Delta$, $\Delta_\mathrm{R} = \Delta e^{i\phi}$, where $\phi$ is the phase difference and $\Delta = |\Delta_\mathrm{L}| = |\Delta_\mathrm{R}|$. Corresponding to the experimental setup, we consider the regime where $|\Delta| \ll U_i$ and $\Gamma_\mathrm{R}, \Gamma_\mathrm{L} \ll U_\mathrm{L}, U_\mathrm{R}, \Delta$ with $\Gamma_i = \pi\nu_\mathrm{F}|t_i|^2$, where $\nu_\mathrm{F}$ is the normal-state density of states in the leads, assumed be constant in the relevant range around the Fermi energy.

### Zero-bandwidth approximation

In the zero-bandwidth approximation (ZBW), one replaces the full BCS lead with a single superconducting impurity:

$$H_{\mathrm{BCS}} \approx H_{\mathrm{ZBW}} = \sum_{i=\mathrm{L,R}} \left( \Delta_i c_{i\uparrow}^\dagger c_{i\downarrow}^\dagger + \Delta_i^* c_{i\downarrow} c_{i\uparrow} \right). \tag{S8}$$

This kind of expansion is in principle uncontrolled in the sense that it is not an expansion in any small parameter and as such its parameters should be regarded as fitting parameters rather than physical parameters.

Within this approximation, the Hamiltonian can be readily diagonalized numerically and from the eigenenergies, $E_i$, the free energy can be found as

$$F(\phi) = k_{\mathrm{B}} T \log \sum_i e^{-E_i/(k_{\mathrm{B}}T)}, \tag{S9}$$

and thereby the supercurrent can be obtained as

$$I(\phi) = \frac{2e}{\hbar} \partial_\phi F(\phi). \tag{S10}$$

From this equation, the critical current is found as $I_{\mathrm{C}} = \max_\phi |I(\phi)|$, which we use to generate the maps of the main article.

One choice of fixing the ZBW parameters is $t_{i,\mathrm{ZBW}} = \sqrt{2\Gamma_i \Delta/\pi}$. This scaling leads to a very good quantitative match between the ZBW approximation and the fourth order perturbation theory for a wide range of parameters and sufficiently small values of $\Gamma_i/U$. A comparison between results from ZBW and fourth order expansion in lead coupling is shown in Fig. S6.

### Perturbative expansion of $I_{\mathrm{C}}$ with BCS leads

Here, we calculate the critical current $I_{\mathrm{C}}$ to the lowest (4th) order in the dot-lead couplings, $t_{\mathrm{L}}$ and $t_{\mathrm{R}}$. In general, the current is calculated as

$$I = i\frac{e}{\hbar} \sum_\sigma \langle [H, n_{\mathrm{R}\sigma}] \rangle = \frac{2e}{\hbar} \operatorname{Im} \sum_\sigma \langle t_{\mathrm{R}} c_{\mathrm{R}\sigma}^\dagger d_{\mathrm{R}\sigma} \rangle, \tag{S11}$$

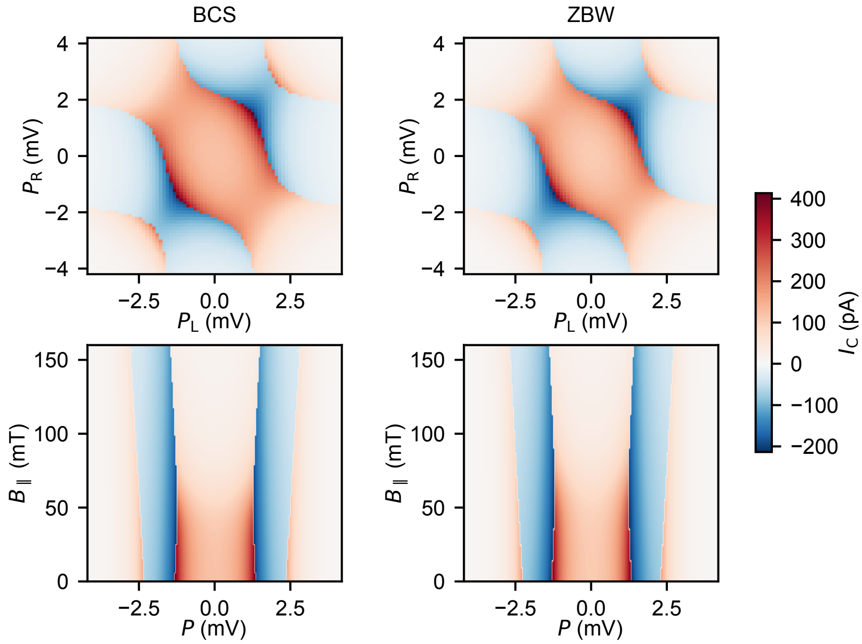


FIG. S6. Comparison of theoretical models of the DQD. a), b) Plots of stability diagrams using fourth order perturbation theory and ZBW approximation, respectively. c), d) B-field line cuts along $P = P_\mathrm{L} = P_\mathrm{R}$ using BCS and ZBW description respectively. Parameters are similar to the main article $\Delta = 200$, $U_\mathrm{L} = 595.25$. $U_\mathrm{R} = 464.84$, $U_\mathrm{C} = 41.41$, $t_0 = 80$, $t_x = 30$, $t_y = t_z = 0$, all in units $\mu$eV, and $g = 15.9$. The charge of the dots are determined through lever arms by $\epsilon_\mathrm{L} = -U_\mathrm{L}/2 - U_\mathrm{C} - \alpha_\mathrm{LL}P_\mathrm{L} - \alpha_\mathrm{LR}P_\mathrm{R}$ and $\epsilon_\mathrm{R} = -U_\mathrm{R}/2 - U_\mathrm{C} - \alpha_\mathrm{RL}P_\mathrm{L} - \alpha_\mathrm{RR}P_\mathrm{R}$ where $\alpha_\mathrm{LL} = 0.2$, $\alpha_\mathrm{LR} = 0.011$, $\alpha_\mathrm{RL} = 0.013$ and $\alpha_\mathrm{RR} = 0.124$. For the fourth order expansion, we use $\Gamma_\mathrm{L} = \Gamma_\mathrm{R} = 33.18$ $\mu$eV, while we use the scaling $t_\mathrm{L,ZBW} = t_\mathrm{R,ZBW} = \sqrt{2\Gamma_\mathrm{L}\Delta/\pi} = 65$ $\mu$eV for the ZBW approximation.

and the lowest order perturbation expansion takes the form

$$\begin{aligned} I &\approx -\frac{2e}{\hbar}\frac{1}{3!}\,\mathrm{Im}\,\frac{1}{\beta}\int_0^\beta \mathrm{d}\tau_1\,\mathrm{d}\tau_2\,\mathrm{d}\tau_3\,\mathrm{d}\tau_4 \sum_\sigma \Big\langle\, \mathrm{T}_\tau\left(H_T(\tau_1)H_T(\tau_2)H_T(\tau_3)t_\mathrm{R}c^\dagger_{\mathrm{R}\sigma}(\tau_4)d_{\mathrm{R}\sigma}(\tau_4)\right)\Big\rangle_0 \\ &= \frac{4e}{\hbar}\Delta^2\Gamma_\mathrm{R}\Gamma_\mathrm{L}\sin\phi\frac{1}{\beta}\int_0^\beta \mathrm{d}\tau_1\,\mathrm{d}\tau_2\,\mathrm{d}\tau_3\,\mathrm{d}\tau_4 f^*(\tau_1-\tau_2)f(\tau_3-\tau_4)B_{ijkl}(\tau_1,\tau_2,\tau_3,\tau_4), \end{aligned} \tag{S12}$$

where $f(\tau) = \sum_{n=-\infty}^{\infty}\frac{e^{-i\omega_n\tau}}{\sqrt{\omega_n^2+\Delta^2}}$ with fermionic Matsubara frequencies $\omega_n = (2n+1)\pi/\beta$ and $\beta = 1/k_\mathrm{B}T$. The label 0 on the expectation value indicates that it is taken with respect to the thermal state of the decoupled dot-lead system. The important object is now

$B_{ijkl}(\tau_1,\tau_2,\tau_3,\tau_4)$ which contains all information about the double dot,

$$B_{ijkl}(\tau_1,\tau_2,\tau_3,\tau_4) = \left\langle \mathrm{T}_\tau \left( d^\dagger_{\mathrm{L}\uparrow}(\tau_1) d^\dagger_{\mathrm{L}\downarrow}(\tau_2) d_{\mathrm{R}\downarrow}(\tau_3) d_{\mathrm{R}\uparrow}(\tau_4) \right) \right\rangle_0 \tag{S13}$$

This object is conveniently evaluated in the basis of eigenstates of $H_0 + H_\mathrm{d} + H_\mathrm{SO}$, obtained numerically for a given parameter set, and the critical current is finally evaluated as $I_\mathrm{C} = I/\sin\phi$, whose sign determines if it is in a 0 or $\pi$ phase.

This result is not used in the main text, and it is included here only as a check of the ZBW calculations in Fig. S6.

## SIGN OF THE CRITICAL CURRENT TO LEADING ORDER IN DOT-LEAD COUPLINGS

In this section, we calculate the sign of $I_\mathrm{C}$ to lowest order in dot-lead couplings, and demonstrate that it is determined from the double-dot ground state, using the simple rule stated in the main text. We start by rewriting Eq. (S12) from the lowest order expansion in lead coupling:

$$\begin{aligned} I_\mathrm{C} &= \int_0^\beta \mathrm{d}\tau_1\,\mathrm{d}\tau_2\,\mathrm{d}\tau_3\,\mathrm{d}\tau_4 g(\tau_1,\tau_2,\tau_3,\tau_4) B(\tau_1,\tau_2,\tau_3,\tau_4) \\ &= \sum_{i,j,k,l=1}^{4} (\epsilon_{ijkl})^2 \int_0^\beta \mathrm{d}\tau_i \int_0^{\tau_i} \mathrm{d}\tau_j \int_0^{\tau_j} \mathrm{d}\tau_k \int_0^{\tau_k} \mathrm{d}\tau_l g(\tau_1,\tau_2,\tau_3,\tau_4) B_{ijkl}(\tau_1,\tau_2,\tau_3,\tau_4), \end{aligned} \tag{S14}$$

which is a sum over all permutations of $\tau_i$'s. Here $g(\tau_1,\tau_2,\tau_3,\tau_4) = 4e/\hbar\Delta^2\Gamma_\mathrm{L}\Gamma_\mathrm{R} f^*(\tau_1 - \tau_2) f(\tau_3-\tau_4)$ and the Levi-Civita symbol is specified with $\epsilon_{1234} = 1$. As we sum over the different permutations of operators in $B_{ijkl}$ it no longer contains any time sorting and can be written as

$$B_{ijkl}(\tau_1,\tau_2,\tau_3,\tau_4) = \epsilon_{ijkl} \Big\langle d_i(\tau_i) d_j(\tau_j) d_k(\tau_k) d_l(\tau_l) \Big\rangle_0, \tag{S15}$$

where $i,j,k,l$ specify the ordering with the definitions $d_1(\tau_1) = d^\dagger_{\mathrm{L}\uparrow}(\tau_1)$, $d_2(\tau_2) = d^\dagger_{\mathrm{L}\downarrow}(\tau_2)$, $d_3(\tau_3) = d_{\mathrm{R}\downarrow}(\tau_3)$ and $d_4(\tau_4) = d_{\mathrm{R}\uparrow}(\tau_4)$. At zero temperature, the dot system is in a definite ground state, $|g\rangle$, of the full dot Hamiltonian and

$$B_{ijkl}(\tau_1,\tau_2,\tau_3,\tau_4) = \epsilon_{ijkl} \langle g|\, d_i U(\tau_i,\tau_j) d_j U(\tau_j,\tau_k) d_k U(\tau_k,\tau_l) d_l \,|g\rangle\,, \tag{S16}$$

where we have separated the trivial time evolution of the isolated dots due to $H_0$ from the evolution generated by $H_\mathrm{d}+H_\mathrm{SO}$, which couples the dots. The time evolution operator above

is defined in the interaction picture as $U(\tau_i,\tau_j) = e^{-(H_0-E_\mathrm{g})\tau_i}\,\mathrm{T}_\tau\, e^{-\int_{\tau_j}^{\tau_i}\mathrm{d}\tau'\bar{H}_\mathrm{d}(\tau')} e^{(H_0-E_\mathrm{g})\tau_j}$ with $\bar{H}_\mathrm{d}(\tau) = e^{H_0\tau}(H_\mathrm{d}+H_\mathrm{SO})e^{-H_0\tau}$, where $\mathrm{T}_\tau$ is the $\tau$-ordering operator.

In Eq. (S14), we expand the time evolution operators appearing in Eq. (S16) to $N$'th order in $\bar{H}_\mathrm{d}$. From now on we will discuss generic contributions to this expansion, which we label $I^{(a,b,c)}_{\mathrm{C},ijkl}$ with $I_\mathrm{C} = \sum_{i,j,k,l=1}^{4}\sum_{a,b,c=0}^{\infty} I^{(a,b,c)}_{\mathrm{C},ijkl}$. The integers $a$, $b$ and $c$ specify the order of expansion (counting from left) of each time evolution operator in Eq. (S16). A single $N$'th order $(a+b+c=N)$ contribution can, in terms of the amplitudes

$$\langle g|\,\mathcal{C}^{(a,b,c)}_{ijkl}\,|g\rangle = \epsilon_{ijkl}(-1)^N \langle g|\, d_i(H_\mathrm{d}+H_\mathrm{SO})^a d_j(H_\mathrm{d}+H_\mathrm{SO})^b d_k(H_\mathrm{d}+H_\mathrm{SO})^c d_l\,|g\rangle \tag{S17}$$

be expressed as,

$$\begin{aligned} I^{(a,b,c)}_{\mathrm{C},ijkl} &= \int_0^\beta d\tau_i \prod_{\mu=0}^{N+2}\left(\int_0^{\tau'_\mu} d\tau'_{\mu+1} e^{-(E_\mu-E_\mathrm{g})(\tau'_\mu-\tau'_{\mu+1})}\right) g(\tau_1,\tau_2,\tau_3,\tau_4)\,\langle g|\,\mathcal{C}^{(a,b,c)}_{ijkl}\,|g\rangle \\ &= \frac{4e}{\hbar}\Gamma_\mathrm{L}\Gamma_\mathrm{R}\,|\Delta|^2 \int_\Delta^\infty \frac{d\omega}{\sqrt{\omega^2-\Delta^2}}\int_\Delta^\infty \frac{d\omega'}{\sqrt{\omega'^2-\Delta^2}} \prod_{m=1}^{n}\left(\frac{1}{E_m-E_\mathrm{g}+\omega+\omega'}\right) \\ &\times \prod_{m'=1}^{n'}\left(\frac{1}{E_{m'}-E_\mathrm{g}+\omega}\right)\prod_{m''=1}^{n''}\left(\frac{1}{E_{m''}-E_\mathrm{g}+\omega'}\right)\prod_{m'''=1}^{n'''}\left(\frac{1}{E_{m'''}-E_\mathrm{g}}\right)\langle g|\,\mathcal{C}^{(a,b,c)}_{ijkl}\,|g\rangle\,, \end{aligned} \tag{S18}$$

with the definition $\tau_i = \tau'_0$, $\tau_j = \tau'_{a+1}$, $\tau_k = \tau'_{a+b+2}$ and $\tau_l = \tau'_{N+3}$. In the second line $n+n'+n''+n''' = N+3$ are positive integers whose values are specified by both the expansion in $a$, $b$ and $c$ and the ordering $ijkl$, while $E_n$ are energies of the uncoupled charge basis $H_0$.

Next comes the critical statement: since all fractions in Eq. (S18) are positive, the sign is determined solely by $\mathcal{C}^{(a,b,c)}_{ijkl}$. For this to be true, the ground state energy of $H_0+H_\mathrm{d}$, $E_\mathrm{g}$, must satisfy that $E_\mathrm{g}\le E_n$ where $E_n$ are eigenenergies of $H_0$. For a hermitian matrix, $A$, with diagonal entries $a_{nn}$ and minimal (maximal) eigenvalues $\lambda_\mathrm{min}$ ($\lambda_\mathrm{max}$), the min-max theorem [5] states that $\lambda_\mathrm{min}\le a_{nn}\le\lambda_\mathrm{max}$. In the charge basis, $H_\mathrm{d}+H_\mathrm{SO}$ only contains off-diagonal elements, and with $A = H_0+H_\mathrm{d}$, we may therefore conclude that $E_\mathrm{g} = \lambda_\mathrm{min} < a_{nn} = E_n$, as needed. Note that this perturbation series breaks down if $E_{m'''} = E_\mathrm{g}$ in the denominator $1/(E_{m'''}-E_\mathrm{g})$. Such a denominator occurs only if $E_{m'''}$ relates to a state with $\pm 2$ electrons compared to the ground state. In such instances one would have to go to higher order in $t_\mathrm{L}$, $t_\mathrm{R}$.

By removing the integrals $\int_\Delta^\infty \frac{\mathrm{d}\omega}{\sqrt{\omega^2-\Delta^2}}$, setting $\omega,\omega' = \Delta$ in the denominators and using $\Gamma_i = \pi t^2_{i,\mathrm{ZBW}}/2\Delta$, one would obtain the corresponding $I_\mathrm{C}$ expansion for a ZBW description

of the superconductors. As such, the previous and following arguments about the sign of $I_\mathrm{C}$ also holds for a ZBW description.

**Sign of all contributions to critical current**

We now turn our attention to the time independent part $\mathcal{C}^{(a,b,c)}_{ijkl}$, which specifies the total sign, and we wish to show that no matter the value of $a, b, c$ or $i, j, k, l$, the sign of a contribution to $I_\mathrm{C}$ is determined by the ground state. In this subsection we neglect spin-orbit coupling, $H_\mathrm{SO}$, the effect of which we discuss in a following subsection.

It is convenient to work in a spin-sorted basis definition of the many-body state $\langle 2,2| = \langle 0| d_{\mathrm{L}\uparrow} d_{\mathrm{R}\uparrow} d_{\mathrm{L}\downarrow} d_{\mathrm{R}\downarrow}$. With this choice, one can make use of the fact that $H_\mathrm{d}$ conserves spin and therefore commutes with operators of opposite spin to sort $\mathcal{C}^{(a,b,c)}_{ijkl}$ as

$$\langle g| \mathcal{C}^{(a,b,c)}_{ijkl} |g\rangle = \sum_{n,m} \alpha_n \alpha_m^* \langle n_\uparrow| \mathcal{C}^{(a_\uparrow b_\uparrow c_\uparrow)}_{\uparrow, i'j'} |m_\uparrow\rangle \langle n_\downarrow| \mathcal{C}^{(a_\downarrow b_\downarrow c_\downarrow)}_{\downarrow, i''j''} |m_\downarrow\rangle \,, \tag{S19}$$

where we have expressed the ground state as a tensor product state between the two spin sectors, $|g\rangle = \sum_n \alpha_n |n_\uparrow\rangle \otimes |n_\downarrow\rangle$, with $\alpha_n$ being prefactors from the diagonalization of $H_0 + H_\mathrm{d}$. The indexes of $\mathcal{C}^{(a_\sigma, b_\sigma, c_\sigma)}_{\sigma, i'j'}$ are specified by the $ijkl$ index as follows: $i', j' \in \{1,4\}$ for spin-up and $i'', j'' \in \{2,3\}$ for spin-down, while ordering is the same as in $ijkl$ for each subset independently, e.g $\mathcal{C}^{(a,b,x)}_{3124}$ corresponds to $\mathcal{C}^{(a_\uparrow, b_\uparrow, c_\uparrow)}_{\uparrow,14}$ and $\mathcal{C}^{(a_\downarrow, b_\downarrow, c_\downarrow)}_{\downarrow,32}$. Finally, the powers $a_\sigma$, $b_\sigma$ and $c_\sigma$ denote the number of $H_\mathrm{d}$ operators containing spin-$\sigma$, such that $\sum_\sigma a_\sigma + b_\sigma + c_\sigma = a + b + c = N$, where we do not permute any operators of same spin in the sorting. This yields the following object, which determines the sign of each spin independently:

$$\langle n_\sigma| \mathcal{C}^{(a_\sigma b_\sigma c_\sigma)}_{\sigma, ij} |m_\sigma\rangle = \epsilon_{ij} (-1)^{a_\sigma + b_\sigma + c_\sigma} \langle n_\sigma| (H_{\mathrm{d}\sigma})^{a_\sigma} d_i (H_{\mathrm{d}\sigma})^{b_\sigma} d_j (H_{\mathrm{d}\sigma})^{c_\sigma} |m_\sigma\rangle \,, \tag{S20}$$

with the Levi-Civita symbols, $\epsilon_{ij}$, defined with $\epsilon_{14} = 1$ and $\epsilon_{23} = 1$.

We will now consider a few specific spin contributions. We start with the state where both dots are void of spin-up electrons such that $|n_\uparrow\rangle = |m_\uparrow\rangle = |0,0\rangle$ where left and right number in the kets refer to the number of spin-up electrons on the left and right dots respectively. Such a contribution yields

$$\begin{aligned} \langle 0,0| \mathcal{C}^{(a_\uparrow b_\uparrow c_\uparrow)}_{\uparrow, ij} |0,0\rangle &= \epsilon_{ij} (-1)^{a_\uparrow + b_\uparrow + c_\uparrow} \langle 0,0| (H_{\mathrm{d}\uparrow})^{a_\uparrow} d_i (H_{\mathrm{d}\uparrow})^{b_\uparrow} d_j (H_{\mathrm{d}\uparrow})^{c_\uparrow} |0,0\rangle \\ &= \delta_{i4} \delta_{j1} \delta_{a_\uparrow 0} \delta_{c_\uparrow 0} \epsilon_{41} (-1)^1 t_0^{b_\uparrow} \langle 0,0| d_{\mathrm{R}\uparrow} d^\dagger_{\mathrm{R}\uparrow} d_{\mathrm{L}\uparrow} d^\dagger_{\mathrm{L}\uparrow} |0,0\rangle \geq 0, \end{aligned} \tag{S21}$$

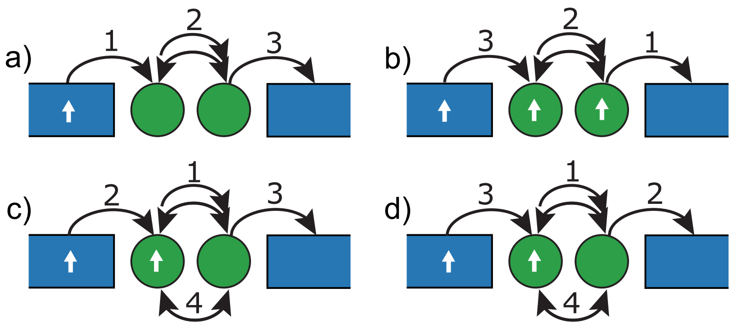


FIG. S7. The paths transferring one electron across the DQD for various ground states. The numbers represent the order of operations applied to $\langle n_\uparrow|$ to reach $|n_\uparrow\rangle$. Lines with arrows in both directions indicate an integer number of back-and-forth jumps each yielding $t_0^2$. a) $|n_\uparrow\rangle = |0,0\rangle$, b) $|n_\uparrow\rangle = |1,1\rangle$ c), one ordering of $|n_\uparrow\rangle = |1,0\rangle$, d) another ordering of $|n_\uparrow\rangle = |1,0\rangle$.

where the disappearance of $H_{\mathrm{d}\uparrow}^{b_\uparrow}$ stems from the fact that the only non-zero contribution arises when $b_\uparrow$ is odd and $H_{\mathrm{d}\uparrow}^{b_\uparrow}$ contains a single $t_0 d_{\mathrm{L}\uparrow}^\dagger d_{\mathrm{R}\uparrow}$ multiplied by $(b_\uparrow - 1)/2$ back-and-forth operators of the type $t_0^2 d_{\mathrm{L}\uparrow}^\dagger d_{\mathrm{R}\uparrow} d_{\mathrm{R}\uparrow}^\dagger d_{\mathrm{L}\uparrow}$. A visual representation of such processes is shown in Fig.S7 a). If the two dots are void of spin-up electrons, the spin-up part will therefore yield a positive sign to Eq. (S19) to all orders of $H_\mathrm{d}$.

Due to the electron-hole symmetry, a very similar derivation follows for the doubly occupied spin-up state

$$\begin{aligned}\langle 1,1|\,\mathcal{C}_{\uparrow,ij}^{(a_\uparrow b_\uparrow c_\uparrow)}\,|1,1\rangle &= \epsilon_{ij}(-1)^{a_\uparrow+b_\uparrow+c_\uparrow}\,\langle 1,1|\,(H_{\mathrm{d}\uparrow})^{a_\uparrow} d_i (H_{\mathrm{d}\uparrow})^{b_\uparrow} d_j (H_{\mathrm{d}\uparrow})^{c_\uparrow}\,|1,1\rangle \\ &= \delta_{i1}\delta_{j4}\delta_{a_\uparrow 0}\delta_{b_\uparrow 0}\epsilon_{14}(-1)^1 t_0^{b_\uparrow}\,\langle 1,1|\, d_{\mathrm{L}\uparrow}^\dagger d_{\mathrm{R}\uparrow}^\dagger d_{\mathrm{L}\uparrow} d_{\mathrm{R}\uparrow}\,|1,1\rangle \geq 0,\end{aligned} \tag{S22}$$

where a visual representation is shown in Fig. S7b.

The odd ground state configurations are a little more complicated, as there is more than one way of organizing operators. Consider contributions with $|n_\uparrow\rangle = |m_\uparrow\rangle = |1,0\rangle$ meaning one spin-up electron on the left dot,

$$\begin{aligned}\langle 1,0|\,\mathcal{C}_{\uparrow,ij}^{(a_\uparrow b_\uparrow c_\uparrow)}\,|1,0\rangle &= \epsilon_{ij}(-1)^{a_\uparrow+b_\uparrow+c_\uparrow}\,\langle 1,0|\,(H_{\mathrm{d}\uparrow})^{a_\uparrow} d_i (H_{\mathrm{d}\uparrow})^{b_\uparrow} d_j (H_{\mathrm{d}\uparrow})^{c_\uparrow}\,|1,0\rangle \\ &= \delta_{b_\uparrow 0} t_0^{a_\uparrow + c_\uparrow}(-1)^1 \Big(\delta_{i1}\delta_{j4}\epsilon_{14}\,\langle 1,0|\, d_{\mathrm{L}\uparrow}^\dagger d_{\mathrm{R}\uparrow} d_{\mathrm{R}\uparrow}^\dagger d_{\mathrm{L}\uparrow}\,|1,0\rangle \\ &\qquad +\delta_{i4}\delta_{j1}\epsilon_{41}\,\langle 1,0|\, d_{\mathrm{R}\uparrow} d_{\mathrm{L}\uparrow}^\dagger d_{\mathrm{R}\uparrow}^\dagger d_{\mathrm{L}\uparrow}\,|1,0\rangle\Big) \\ &\leq 0,\end{aligned} \tag{S23}$$

which shows that all such non-zero contributions are negative. By symmetry, exchanging spin-up with spin-down yields precisely the same signs. Similar calculations can be done for the other configurations and here we list the results:

$$\langle 0,1|\,\mathcal{C}^{(a_\sigma b_\sigma c_\sigma)}_{\sigma,ij}\,|0,1\rangle \leq 0, \tag{S24a}$$

$$\langle 1,0|\,\mathcal{C}^{(a_\sigma b_\sigma c_\sigma)}_{\sigma,ij}\,|0,1\rangle \geq 0, \tag{S24b}$$

$$\langle 0,1|\,\mathcal{C}^{(a_\sigma b_\sigma c_\sigma)}_{\sigma,ij}\,|1,0\rangle \geq 0. \tag{S24c}$$

With these results it is straightforward to compute the sign of the critical current for a given ground state using Eq. (S19). Here we will show some results to illustrate the methodology:

$$\langle 0,0|\,\mathcal{C}^{(a,b,c)}_{ijkl}\,|0,0\rangle = \langle 0,0|\,\mathcal{C}^{(a_\uparrow b_\uparrow c_\uparrow)}_{\uparrow,ij}\,|0,0\rangle\,\langle 0,0|\,\mathcal{C}^{(a_\downarrow b_\downarrow c_\downarrow)}_{\downarrow,ij}\,|0,0\rangle \geq 0 \tag{S25a}$$

$$\langle 2,2|\,\mathcal{C}^{(a,b,c)}_{ijkl}\,|2,2\rangle = \langle 1,1|\,\mathcal{C}^{(a_\uparrow b_\uparrow c_\uparrow)}_{\uparrow,ij}\,|1,1\rangle\,\langle 1,1|\,\mathcal{C}^{(a_\downarrow b_\downarrow c_\downarrow)}_{\downarrow,ij}\,|1,1\rangle \geq 0 \tag{S25b}$$

$$\langle \uparrow,0|\,\mathcal{C}^{(a,b,c)}_{ijkl}\,|\uparrow,0\rangle = \langle 1,0|\,\mathcal{C}^{(a_\uparrow b_\uparrow c_\uparrow)}_{\uparrow,ij}\,|1,0\rangle\,\langle 0,0|\,\mathcal{C}^{(a_\downarrow b_\downarrow c_\downarrow)}_{\downarrow,ij}\,|0,0\rangle \leq 0 \tag{S25c}$$

$$\langle 2,\uparrow|\,\mathcal{C}^{(a,b,c)}_{ijkl}\,|2,\uparrow\rangle = \langle 1,1|\,\mathcal{C}^{(a_\uparrow b_\uparrow c_\uparrow)}_{\uparrow,ij}\,|1,1\rangle\,\langle 1,0|\,\mathcal{C}^{(a_\downarrow b_\downarrow c_\downarrow)}_{\downarrow,ij}\,|1,0\rangle \leq 0 \tag{S25d}$$

What we have shown is that, independent of ordering and order of $H_{\rm d}$, all contributions to $I_{\rm C}$ in Eq. (S18) have the same sign, proving that the signs shown above must also be the sign of $I_{\rm C}$ for the respective ground states. This method can also be used to compute the sign of $I_{\rm C}$ for ground states that are not eigenstates of $H_0$, but eigenstates of $H_0 + H_{\rm d}$. Consider for example the ground state with a single electron delocalized across the dots, $|\uparrow\rangle = a\,|\uparrow,0\rangle - b\,|0,\uparrow\rangle$, where $a$ and $b$ have the same sign. Then it follows that

$$\begin{aligned}\langle\uparrow|\,\mathcal{C}^{(a,b,c)}_{ijkl}\,|\uparrow\rangle = \langle 0,0|\,\mathcal{C}^{(a_\downarrow b_\downarrow c_\downarrow)}_{\downarrow,ij}\,|0,0\rangle \Big(& a^2\,\langle 1,0|\,\mathcal{C}^{(a_\uparrow b_\uparrow c_\uparrow)}_{\uparrow,ij}\,|1,0\rangle + b^2\,\langle 0,1|\,\mathcal{C}^{(a_\uparrow b_\uparrow c_\uparrow)}_{\uparrow,ij}\,|0,1\rangle \\ & -ab\,\langle 1,0|\,\mathcal{C}^{(a_\uparrow b_\uparrow c_\uparrow)}_{\uparrow,ij}\,|0,1\rangle - ab\,\langle 0,1|\,\mathcal{C}^{(a_\uparrow b_\uparrow c_\uparrow)}_{\uparrow,ij}\,|1,0\rangle\Big) \\ \leq 0,&\end{aligned} \tag{S26}$$

which proves that the sign of $I_{\rm C}$ in the single electron doublet sector is negative to all orders in $t_0$. Using the same methodology on other ground states, we find:

$$\langle\uparrow\downarrow|\,\mathcal{C}^{(a,b,c)}_{ijkl}\,|\uparrow\downarrow\rangle \geq 0, \tag{S27a}$$

$$\langle\sigma|\,\mathcal{C}^{(a,b,c)}_{ijkl}\,|\sigma\rangle \leq 0, \tag{S27b}$$

$$\langle\uparrow\downarrow\sigma|\,\mathcal{C}^{(a,b,c)}_{ijkl}\,|\uparrow\downarrow\sigma\rangle \leq 0, \tag{S27c}$$

$$\langle\uparrow\uparrow|\,\mathcal{C}^{(a,b,c)}_{ijkl}\,|\uparrow\uparrow\rangle \geq 0, \tag{S27d}$$

for eigenstates of $H_0 + H_\mathrm{d}$ with electrons delocalized across the dots:

$$|{\uparrow\downarrow}\rangle = a\,|{\uparrow},{\downarrow}\rangle + b\,|{\downarrow},{\uparrow}\rangle - c\,|2,0\rangle - d\,|0,2\rangle\,, \tag{S28a}$$

$$|{\uparrow\downarrow}\;\sigma\rangle = f\,|2,\sigma\rangle - g\,|\sigma,2\rangle\,, \tag{S28b}$$

defined with positive prefactors, $a, b, c, d, f, g$, on all components.

Crucially for this experiment, we have shown that both a triplet ground state, $|{\uparrow\uparrow}\rangle$, and a singlet ground state, $|{\uparrow\downarrow}\rangle$, will guarantee a positive $I_\mathrm{C}$. This concludes the proof that for the serial double dot, neglecting spin-orbit coupling, the sign of $I_\mathrm{C}$ to lowest order in dot-lead couplings is completely determined by the charge ground state.

Even though these derivations are quite technical, the results can be summarized as a rather simple rule: For each spin in a Cooper pair in the left lead, count the number of same-spin dot electrons it crosses to get from left to right lead. For each such same-spin crossing attribute a minus sign. The sign of $I_\mathrm{C}$ will then be equal to the product of all such crossing signs. This rule can be inferred from Eqs. (S19) and (S24), noticing that for a delocalized ground state all contributions yield the same sign as resulting from one of its localized constituents. For a serial double dot this rule clearly implies that the sign of $I_\mathrm{C}$ is determined by the total charge parity of the dots: the sign is negative for odd parity and positive for even parity, regardless of the spin configuration.

**Discussion of spin-orbit coupling**

So far we have established that the sign of the critical current for a double dot without spin-orbit coupling can be inferred solely from the ground state. In this subsection, we discuss the possible implications of a finite spin-orbit coupling on the two quantum dots, implemented as a spin-dependent interdot tunneling amplitude. We begin by considering only the spin-conserving tunnel coupling, $t_z$, and write the total interdot tunneling Hamiltonian as

$$\begin{aligned} H_\mathrm{d} + H_\mathrm{SO} &= \sum_\sigma \Big( (t_0 + i\sigma t_z) d^\dagger_{\mathrm{L}\sigma} d_{\mathrm{R}\sigma} + \mathrm{h.\,c} \Big) \\ &= t_\mathrm{eff} \sum_\sigma \Big( e^{i\sigma\theta} d^\dagger_{\mathrm{L}\sigma} d_{\mathrm{R}\sigma} + \mathrm{h.\,c} \Big)\,, \end{aligned} \tag{S29}$$

where $t_\mathrm{eff}$ is the modulus and $\theta$ the complex phase of $t_0 + it_z$. On this system we can perform a gauge transformation $e^{i\sigma\theta} d^\dagger_{\mathrm{L}\sigma} = \tilde{d}^\dagger_{\mathrm{L}\sigma}$ which removes $\theta$ from the interdot coupling and moves

it onto the left dot-lead tunneling amplitude:

$$H_{TL} = t_{\mathrm{L}} \sum_{k\sigma} \left( e^{i\sigma\theta} c^{\dagger}_{\mathrm{L}k\sigma} \tilde{d}_{\mathrm{L}\sigma} + \mathrm{h.\,c} \right). \tag{S30}$$

Since the expansion in $t_{\mathrm{L}}$, $t_{\mathrm{R}}$ in Eq. (S12) contains two electrons of opposite spin jumping from the superconductor lead to the dot, this phase cancels out in $I_{\mathrm{C}}$, and the only effect of $t_z$ is simply to renormalize the interdot coupling $t_{\mathrm{eff}} = \sqrt{t_0^2 + t_z^2}$, leaving the sign of $I_{\mathrm{C}}$ unchanged.

Including either $t_x$ or $t_y$, interdot tunnelling is no longer spin conserving, and therefore disrupts the spin-sorted arguments used above to show that all contributions to $I_{\mathrm{C}}$ have the same sign. This is most easily illustrated with an example. Consider a specific term arising from the combination $H_{\mathrm{SO}} H_{\mathrm{d}} H_{\mathrm{SO}}$ with a finite $t_y$:

$$H_{\mathrm{SO}} H_{\mathrm{d}} H_{\mathrm{SO}} = -t_y^2 t_0 d^{\dagger}_{\mathrm{L}\uparrow} d_{\mathrm{R}\downarrow} d^{\dagger}_{\mathrm{R}\downarrow} d_{\mathrm{L}\downarrow} d^{\dagger}_{\mathrm{L}\downarrow} d_{\mathrm{R}\uparrow} + \ldots \tag{S31}$$

When acting on $|0, \uparrow\rangle$, this operator is equivalent to $-t_y^2 H_{\mathrm{d}}$. Such combinations of operators will arise in Eq. (S17), where, for example, a contribution with $a = 1$ would contain $H_{\mathrm{d}}$ while a contribution with $a = 3$ would contain $H_{\mathrm{SO}} H_{\mathrm{d}} H_{\mathrm{SO}}$. As these two terms will have different signs, we observe that not all contributions to $I_{\mathrm{C}}$ have the same sign.

Without any external magnetic field, one may choose the spin quantization axis to be aligned with the spin-orbit field, such that only $t_z$ is non-zero. As such the sign of $I_{\mathrm{C}}$ is still completely determined by the ground state of the DQD. With a finite external magnetic field, however, $t_x$ and $t_y$ components are unavoidable unless the field is carefully aligned with the spin-orbit field. In this case, $I_{\mathrm{C}}$ will sample amplitudes of different signs and the overall sign of $I_{\mathrm{C}}$ cannot be guaranteed analytically, since the magnitudes of the individual terms now also matter. Instead, we have done this numerically to confirm the observed signs of $I_{\mathrm{C}}$ in the plots presented in the main text. To lowest order in $H_{\mathrm{d}}$ and $H_{\mathrm{SO}}$, it can be shown analytically, that the sign of $I_{\mathrm{C}}$ remains determined by the ground state, and that it is only higher order terms including both $H_{\mathrm{d}}$ and $H_{\mathrm{SO}}$, such as Eq.(S31), which yield contributions of different signs. To leading order, the sign of $I_{\mathrm{C}}$ thus remains determined by the ground state.

## SIMPLE ARGUMENTS FOR TRIPLET BLOCKADE

In the main text, the key quantity is the critical current in a double-dot Josephson junction that is tuned to the (1,1) charge configuration. We use the term *triplet blockade* for the effect that the critical current in this setup is suppressed when the ground state is tuned from a singlet configuration to a triplet configuration.

Here, we provide simple arguments for a strong triplet blockade in two different limiting cases: the large-gap limit, $\Delta \gg U$, and the strong-Coulomb-repulsion limit, $U \gg \Delta$. We also outline a process-counting argument that supports *partial* triplet blockade in the intermediate regime $\Delta \sim U$.

For the simple arguments, we make a number of simplifying assumptions. (1) We disregard the interdot Coulomb repulsion $U_C$. (2) Instead of the proper singlet ground state, we address the case when the ground state holds a spin-up electron in the left dot and a spin-down electron in the right dot (the *up-down* state), (3) We describe the leads within the zero-bandwidth (ZBW) approximation. (4) We describe the Josephson current to leading order in dot-lead as well as inter-dot tunnel amplitude, assuming these to be small compared to the superconducting gap $\Delta$ and the on-site Coulomb repulsion $U$. With these simplifications, the leading-order (6th order) Josephson current can be described as a sum of contributions, where each term can be visualized as a six-step process in which a Cooper pair from one lead is transported over to the other lead. Four exemplary processes are shown in Fig. S8. The intermediate states of such processes are virtual states, in the sense that they have a high energy, either due to quasiparticle excitations, or due to Coulomb repulsion.

First, we revisit the case of the large-gap limit $\Delta/U \gg 1$, which was described in Ref. [6, 7]. In this case, the reason for the triplet blockade is that a triplet ground state allows only such processes whose intermediate states have one or two quasiparticles in the leads. One example is shown in Fig. S8b. In the 6th-order perturbative description of the ZBW model, the contribution of these processes scales as $\sim \Delta^{-5}$. In contrast, the up-down state allows for intermediate states where there are no quasiparticles in the leads; an example is shown in Fig. S8a, where the 2nd, 4th and 6th states of the diagram do not have any quasiparticles. As a consequence, the contribution of such processes scale as $\sim \Delta^{-2}$. In conclusion, in the large-gap regime the ratio of the triplet and up-down critical currents is suppressed by $\Delta^{-3}$, leading to a strong triplet blockade.

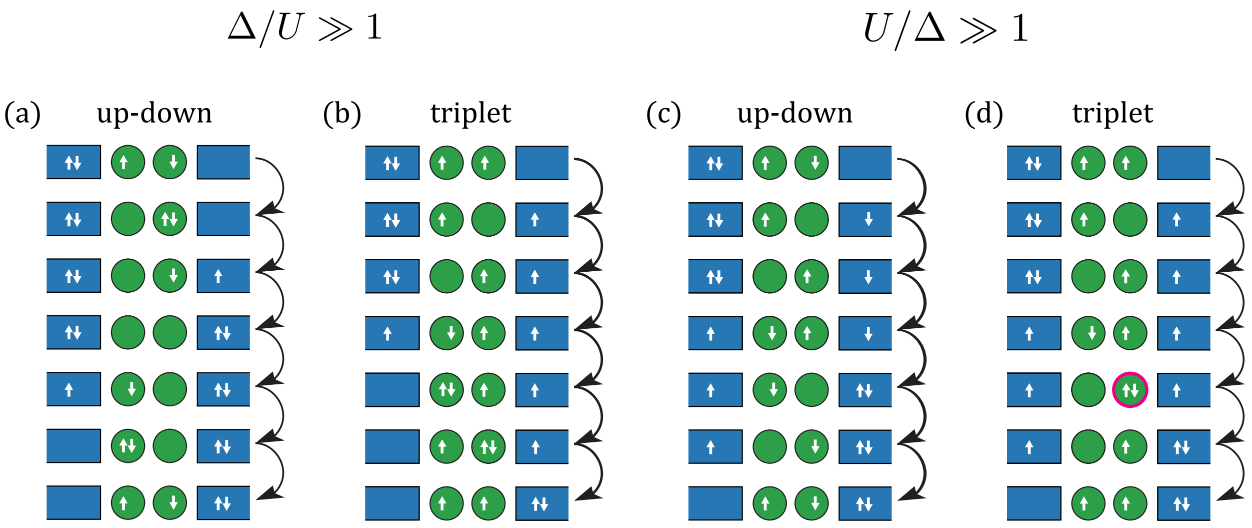


FIG. S8. Example processes contributing to the Josephson current through the double dot. (a) Up-down process with intermediate states lacking quasiparticles, hence less penalized by a large gap $\Delta \gg U$. (b) Triplet process with intermediate states that all have at least one quasiparticle, hence more penalized by $\Delta$. (c) Up-down process with all states having at most singly occupied quantum dots, hence exempt from Coulomb energy penalty. (d) Triplet process with an intermediate state that has a doubly occupied quantum dot and hence energetically penalized in the $U \gg \Delta$ regime.

Now let us turn to the strong-Coulomb-repulsion limit $U/\Delta \gg 1$. Consider a point in the charge stability diagram in the vicinity of the boundary of the single-electron region and the (1,1) region. In this case, any intermediate state that has a DQD occupation different from 1 and 2 has a large energy penalty in the corresponding energy denominator, and hence is strongly suppressed. In addition, among the processes where all states have DQD occupation 1 or 2, the ones involving a doubly occupied quantum dot also come with a large Coulomb energy penalty and hence are also suppressed.

Importantly, in the processes allowed by the triplet ground state, there is at least one intermediate state that has a doubly occupied quantum dot; for example, see Fig. S8d, where the right dot is doubly occupied in the 5th state. The critical current of the triplet will therefore scale as $\sim U^{-1}$. In contrast, for an up-down ground state, there is a process where the intermediate states have only singly occupied quantum dots, see Fig. S8c. The contribution of this process to the critical current will scale as $\sim U^{0}$. In conclusion, in the strong-Coulomb-repulsion regime the ratio of the triplet and up-down critical currents is suppressed as $U^{-1}$, again leading to a strong triplet blockade.

Even though we have argued for a strong triplet blockade in both limiting cases $\Delta \gg U$ and $U \gg \Delta$, it is in principle possible that the triplet critical current exceeds the up-down critical current in the intermediate regime $U \sim \Delta$. Here, we argue that this is not the case. In this regime, we estimate the ratio of the triplet and up-down critical currents from the ratio of the total number of 6th-order process. In the triplet case, the total number of allowed processes is 80, whereas the up-down state allows 320 processes in total, leading to a rough estimate of the critical current ratio of 0.25. Note that the actual critical current ratio also depends on the amplitudes of every process. Due to this estimate, we expect a partial triplet blockade in this intermediate regime.

Finally, we comment on the validity of the simplifying assumptions (1), (2) and (3) above. (1) The above considerations generalize as long as the interdot Coulomb repulsion energy $U_C$ is moderate. The analysis of the strong-Coulomb-repulsion regime could change, e.g., if $U_C$ would be a parameter tied to $U$, e.g., $U_C = U/2$, but that is beyond the scope of this work. (2) The above arguments generalize to the case when a singlet ground state is considered, instead of the up-down state. One result that is changed is the order-of-magnitude estimate of the critical current ratio in the intermediate regime $U \sim \Delta$: counting the processes of the singlet ground state yields a ratio of $80/1120 \approx 0.07$, which is even smaller than the estimate $80/320 = 0.25$ quoted above. (3) The above considerations generalize to the model with BCS leads. One technical difference is that in that model, quasiparticles have not only a spin quantum number, but also a momentum quantum number, and the contributions visualized in Fig. S8 have to be summed (or integrated) with respect to the quasiparticle momentum. The main difference occurring from this is that processes from BCS leads will scale with an additional $\Delta^2$ factor which can also be accounted for in the choice of $t_{i,\mathrm{ZBW}}$. Nevertheless the $\Delta$ ratios between different processes are the same and as such the above blockade arguments also hold for BCS leads.

## SUPPLEMENTARY REFERENCES


[1] K. Flöhr, M. Liebmann, K. Sladek, H. Y. Günel, R. Frielinghaus, F. Haas, C. Meyer, H. Hardtdegen, T. Schäpers, D. Grützmacher, *et al.*, Review of scientific instruments **82**, 113705 (2011).

[2] W. G. Van der Wiel, S. De Franceschi, J. M. Elzerman, T. Fujisawa, S. Tarucha, and L. P. Kouwenhoven, Reviews of Modern Physics **75**, 1 (2002).

[3] J. C. Estrada Saldaña, A. Vekris, G. Steffensen, R. Žitko, P. Krogstrup, J. Paaske, K. Grove-Rasmussen, and J. Nygård, Physical Review Letters  (2018).

[4] J. Danon and Y. V. Nazarov, Phys. Rev. B **80**, 041301 (2009).

[5] K. F. Riley and M. P. Hobson, Essential mathematical methods for the physical sciences (Cambridge University Press, 2011) p. 66.

[6] C. Karrasch, S. Andergassen, and V. Meden, Physical Review B **84**, 134512 (2011).

[7] S. Droste, S. Andergassen, and J. Splettstoesser, Journal of Physics: Condensed Matter **24**, 415301 (2012).
